# Supplementary material for: A Comprehensive Survey of Advanced Persistent Threat Attribution: Taxonomy, Methods, Challenges and Open Research Problems
Source: arXiv:2409.11415 source file (2024-10-06)
Supplement: Supplementary file 1 [file Appendix.tex]

\input{Table/ArtifactComparisonExplaination}
